# Supplementary material for: Femtosecond switching of strong light-matter interactions in microcavities with two-dimensional semiconductors
Source: arXiv:2408.00111 ancillary file (2024-07-31)
Supplement: Supplementary file 1 [file Genco_et_al_SI.pdf]

# Femtosecond switching of strong light-matter interactions in microcavities with two-dimensional semiconductors - *Supplementary Information*

Armando Genco,[1,*] Charalambos Louca,[1,2,*] Cristina Cruciano,[1] Kok Wee Song,[3] Chiara Trovatello,[1,4] Giuseppe Di Blasio,[1] Giacomo Sansone,[5] Sam Randerson,[6] Peter Claronino,[6] Rahul Jayaprakash,[6] Kenji Watanabe,[7] Takashi Taniguchi,[7] David G. Lidzey,[6] Oleksandr Kyriienko,[3] Stefano Dal Conte,[1] Alexander I. Tartakovskii,[6,†] and Giulio Cerullo[1,8,‡]

[1]*Dipartimento di Fisica, Politecnico di Milano,*
*Piazza Leonardo Da Vinci 32, 20133 Milano, Italy*
[2]*NanoPhotonics Centre, Cavendish Laboratory,*
*Department of Physics, JJ Thompson Ave,*
*University of Cambridge, Cambridge, UK*
[3]*Department of Physics, University of Exeter, Stocker Road, EX4 4PY, Exeter, UK*
[4]*Department of Mechanical Engineering, Columbia University, New York, NY 10027, USA*
[5]*Dipartimento di Scienze Matematiche, Fisiche e Informatiche,*
*Università di Parma, Parco Area delle Scienze 7/A, 43124 Parma, Italy*
[6]*Department of Physics and Astronomy, University of Sheffield, Hounsfield Road, S3 7RH, Sheffield, UK*
[7]*Advanced Materials Laboratory, National Institute for*
*Materials Science, 1-1 Namiki, Tsukuba, 305-0044, Japan*
[8]*CNR-IFN, Piazza Leonardo da Vinci 32, Milano, 20133, Italy*

(Dated: July 31, 2024)

## SUPPLEMENTARY NOTE S1: ULTRAFAST BEHAVIOUR OF MONOLAYER EXCITONS

We performed pump-probe spectroscopy experiments at low temperature (8K) on a $MoS_2$ ML encapsulated in hBN and placed on a DBR, to compare the excitons dynamics with the ones measured in the $MoS_2$ BL. For this experiment, we used broadband probe pulses and narrow band pump pulses (10 nm), the latter tuned at the energy of the intralayer A excitons ($\approx$ 1.94 eV), in a similar configuration to the measurements on $MoS_2$ BL shown in Fig.1 of the main text. We also pumped the ML with the same fluence used for the BL experiments (5 $\mu Jcm^{-2}$). Figure S1a shows the transient reflectivity map of the ML exhibiting a strong signal at the intralayer exciton energy. This system does not support interlayer excitons being made of a single TMD monolayer.

We extracted the intralayer exciton dynamics from the transient reflectivity data following the procedure described in the main text for the BL measurements, i.e. tracing the variation of the

exciton peak from the dynamic RC. Fig. S1b shows the resulting exciton population dynamics, which follow an initial ultrafast build-up, when the pump pulse excites the sample, and a double exponential decay. The first sub-ps decay is related to bright excitons direct relaxation processes, while the second longer decay is attributed to slow exciton scattering from dark states. We observe that compared to the BL exciton dynamics, here the slow decay component is much more prominent, effectively extending the exciton population for longer times. In fact, the exciton density at 10 ps is still about 70% of the initial one. This difference compared to the BL case is probably due to the presence in the latter of fast non-radiative charge relaxation channels from K points to the energy minima of the band structure, typical of indirect bandgap semiconductors [1, 2], which limit the overall exciton lifetime.

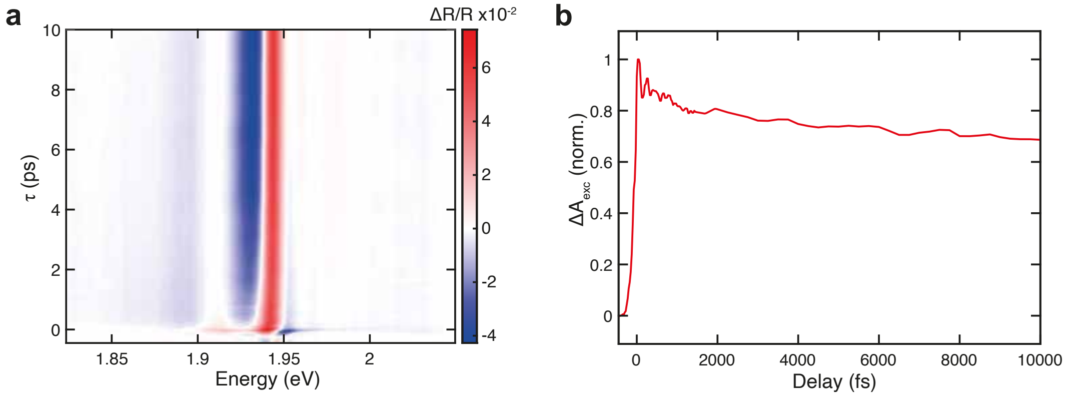


Supplementary Figure S1. a) Transient differential reflectivity color map as a function of pump-probe delay time $\tau$ and photon energy measured for $MoS_2$ ML. b) Normalized peak amplitude variation ($\Delta A_{\mathrm{exc}}$) of $X_{\mathrm{A-ML}}$, extracted from the dynamic RC at different time delays.

## SUPPLEMENTARY NOTE S2: MONOLAYER CAVITY DISPERSION

Fig. S2 shows the reflectivity dispersion of a monolayer $MoS_2$ embedded in a microcavity. A clear anticrossing around the exciton energy is observed, resulting in lower and upper polariton branches (LPB, UPB). The RC spectra are fitted with Lorentzian functions for each angle.

A fit of the extracted peak energies with the Hamiltonian of two coupled oscillators is performed, such that $H_{\mathrm{ML}} = \begin{pmatrix} E_{\mathrm{c}} & \Omega_{\mathrm{A_{ML}}} \\ \Omega_{\mathrm{A_{ML}}} & E_{\mathrm{A_{ML}}} \end{pmatrix}$, where $E_{\mathrm{c}}$ and $E_{\mathrm{A_{ML}}}$ are the energies of the cavity mode and A exciton, respectively. The extracted value of Rabi splitting, $\Omega_{\mathrm{A_{ML}}}$ was $28.5 \pm 0.3$ meV. The A exciton energy is $1.948 \pm 0.001$ eV. The results of the fit are shown in Fig. S2b.

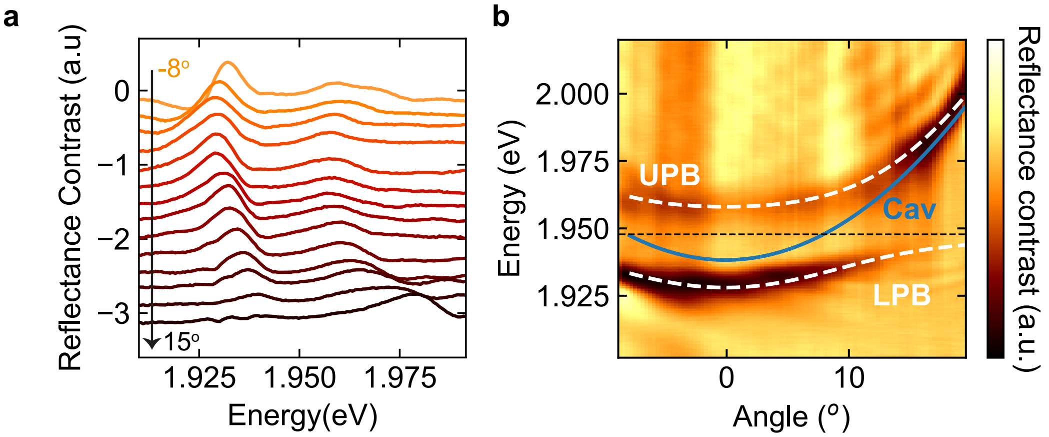


Supplementary Figure S2. a) Waterfall plot of the RC spectra as a function of angle for ML $MoS_2$ embedded in a microcavity. b) Energy-angle map of the cavity reflectivity spectra. The fitted upper and lower polariton branches (UPB, LPB) are shown as white dashed curves. The black horizontal dashed line corresponds to the $X_A$ energy. The cavity mode (Cav) is shown as a blue solid curve.

## SUPPLEMENTARY NOTE S3: BILAYER CAVITY TRANSIENT DIFFERENTIAL REFLECTIVITY

Fig. S3 shows the transient differential reflectivity map of the bilayer $MoS_2$ embedded in a microcavity, used to extract the plots in Fig.2 of the main paper, together with some spectral cross-sections taken at different time delays.

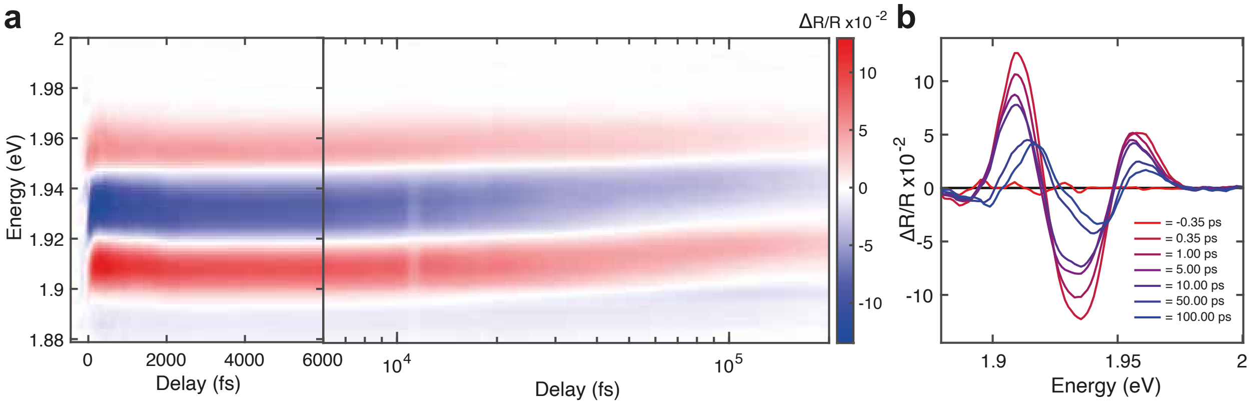


Supplementary Figure S3. a) Transient differential reflectivity color map as a function of pump-probe delay time $\tau$ and photon energy measured for the $MoS_2$ BL cavity. b) Spectral cross-section of the map in (a) taken at different time delays.

## SUPPLEMENTARY NOTE S4: SC SWITCHING IN ML CAVITIES

In this section, we discuss the results of the excitation of a $MoS_2$ ML cavity in SC regime with ultrafast pump pulses tuned at $\approx 1.94$ eV, with an energy of 3.75 pJ (212.2 $\mu J cm^{-2}$). Figure S4a shows the relative transmittance spectra of the cavity probed as a function of the delay time between pump and probe pulses.

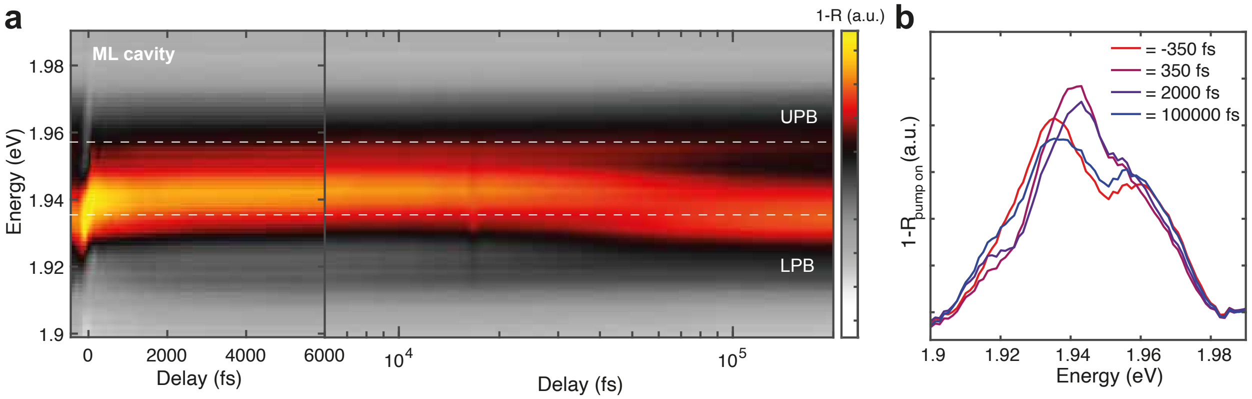


Supplementary Figure S4. a) Color map of the 1-R spectra of the ML microcavity as a function of the pump-probe delay showing the collapse and later revival of the UPB and LPB (white dashed lines). b) 1-R spectra of the ML microcavity taken at different pump-probe delays, extracted from panel (a).

Similarly to the BL cavity case, we observed a strong modulation of the UPB and LPB energies due to optical saturation of excitons, reaching a full collapse into a weakly coupled cavity mode. This proves that exciton nonlinearities in MLs are also strong enough to allow a switching of the SC regime. However, differently from the BL cavity, the recovery of SC is much slower, failing to produce a full switching cycle within 1 ps. This is due to the slower depopulation mechanisms for excitons in MLs, exhibiting overall a much slower decay compared to BLs, as discussed in Supplementary Note S1. We note that we used the same pump fluence of the experiments on the BL cavity shown in Fig.2 of the main text, which in that case led to an ultrafast complete switching cycle. On the other hand, decreasing the excitation fluence in the ML cavity to achieve the same result will not lead to a complete quenching of SC, but just a partial contraction of the Rabi splitting, due to an insufficiently high peak polariton density.

The $on/off$ contrast in this case is worse than what achieved in the BL cavity, looking at the 1-R spectra at different delays in Fig. S4b, extracted from the map in the same figure. This is a consequence of the smaller Rabi splitting obtained in this system (see Supplementary Note S2), which is only slightly larger than the exciton linewidth, broadened by excitation-induced dephasing

[3, 4].

## SUPPLEMENTARY NOTE S5: TRANSFER MATRIX SIMULATIONS

In order to perform the simulations of the BL cavity optical response increasing the exciton density (Fig.3 of the main text) we used the Transfer Matrix Method (TMM) [5, 6]. With this theoretical approach, it is possible to calculate with high accuracy the reflectance, absorbance and transmittance of a multi-layer thin film optical structure, knowing the thicknesses and the complex refractive indexes of the layers. This method can be applied very well also to planar microcavities in SC regime [7]. For the layers of the DBR, PMMA spacer and silver mirrors, we used tabulated values of refractive index (http://refractiveindex.info). For the hBN we assumed a constant refractive index of 1.85 [8], while we calculated the refractive index of the TMD fitting the experimental RC, using the Kramers-Kronig (KK) method [9, 10]. In particular, we used two Lorentzian functions to fit the excitonic optical response for $X_{A-BL}$ and hIX, while we kept fixed the high frequency dielectric constant $\epsilon_\infty$ at 25 [11].

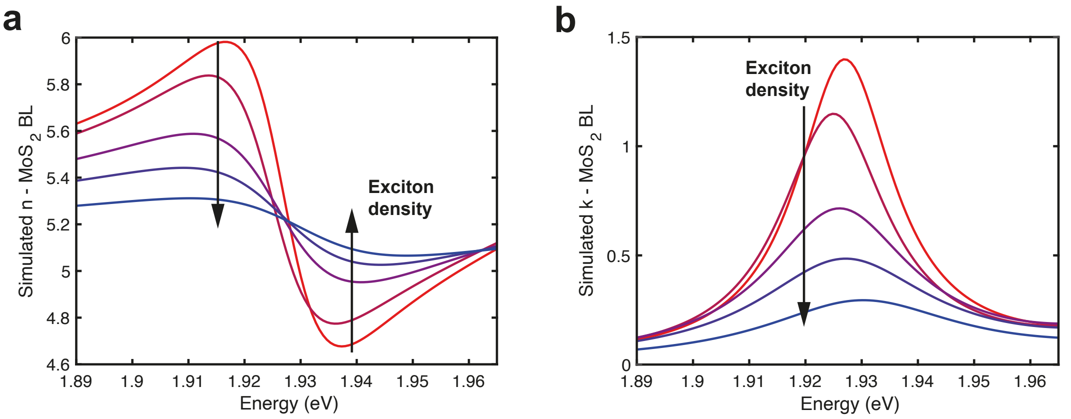


Supplementary Figure S5. a) Real part of the complex refractive index (n) of a $MoS_2$ BL calculated for an increasing exciton density, used in the TMM calculations of the microcavity optical response. b) Imaginary part of the complex refractive index (k) of a $MoS_2$ BL calculated for an increasing exciton density, used in the TMM calculations of the microcavity optical response.

To take into account the effects of the increased exciton density on the absorption bleaching, energy shift and spectral broadening of the exciton features, we fitted the experimental RC spectra of an out-of-cavity $MoS_2$ BL measured at different laser fluences in single narrowband ultrashort pulse experiments, reported in one of our previous works [12]. The real and imaginary part of the refractive index of the $MoS_2$ BL resulting from the KK analysis at different exciton densities

are shown in Fig. S5. Using such density-dependent TMD optical constants, we found a good match between the experimental and calculated cavity 1-R spectra in Fig.3 of the main text, for increasing exciton densities of $1{*}10^4$, $2{*}10^4$, $3.5{*}10^4$, $5{*}10^4$ and $8{*}10^4$ $\mu m^{-2}$. We note that here we make the assumption of attributing the SC collapse mainly to the effect of the optical saturation of excitons, without taking into account other polaritonic effects in our simulations.

## SUPPLEMENTARY NOTE S6: THEORY ON OPTICAL SATURATION IN $MOS_2$ BL CAVITIES

### The spectrum of the probe field

In the experiment, the intralayer exciton ($X_{A-BL}$) in a bilayer $MoS_2$ is probed. The Hamiltonian of the probed exciton and microcavity coupled system can be written as

$$H = \begin{bmatrix} E_c - i\kappa & \frac{1}{2}g(n_X)\Omega_{A_{BL}} \\ \frac{1}{2}g(n_X)\Omega_{A_{BL}} & E_{A_{BL}} - i\gamma \end{bmatrix} \tag{S1}$$

where the $E_c$ is the cavity-photon energy and $E_{A_{BL}}$ is the $X_{A-BL}$ (probed) exciton energy. The cavity-photon and the probed exciton linewidth are $\kappa$ and $\gamma$ respectively. The nonlinear saturation in the arbitrary order can be written as

$$g(n_X) = e^{-\alpha n_X}, \tag{S2}$$

and it depends on the total density of exciton $n_X$ in $MoS_2$. This includes bright and dark excitonic fractions, as saturation comes from Pauli statistical effects and relies on the presence of fermionic constituents. The factor $g(n_X)$ renormalizes the Rabi splitting such that coupling decreases in the presence of electrons and holes. The parameter $\alpha$ depends on the details of the exciton wavefunction. The estimation of $\alpha$ is outlined in Ref. [13].

The optical response of the cavity with bilayer $MoS_2$ embedded is determined by the polariton density of states $[\Xi(\omega)]$ which is given by the imaginary part of the photonic Green's function $\Xi(\omega) = \mathrm{Im}[G_c(\omega)]$. The full Green's function is

$$G(\omega) = [\omega - H]^{-1} = \begin{bmatrix} G_c(\omega) & D(\omega) \\ D^*(\omega) & G_X(\omega) \end{bmatrix} \tag{S3}$$

and the photonic part is the diagonal matrix element in $G(\omega)$ matrix located at the top left corner that we denote as $G_c(\omega)$. In this formalism, the hybridization of a polariton can be understood as the photon dressed by the excitons.

In the next section, we investigate $\Xi(\omega)$ under different pumping conditions. The formation of the excitonic occupation is determined by how the system is excited initially. This will lead to different time-dependent optical responses.

## Time-evolution of the exciton density

To model the time-dependent total exciton density, we write the rate equation for the long-lived excitons ($n_\mathrm{R}$) and the excitons created by pumping ($n_\mathrm{p}$) as

$$\frac{dn_\mathrm{p}}{dt} = -\gamma_\mathrm{p} n_\mathrm{p} - r n_\mathrm{p} + \Theta(t), \tag{S4}$$

$$\frac{dn_\mathrm{R}}{dt} = -\gamma_\mathrm{R} n_\mathrm{R} + r n_\mathrm{p}, \tag{S5}$$

where $\gamma_\mathrm{p}$ is the pumped exciton decay rate, and $r$ is the transfer rate from bright to dark excitons. For the pumping, we may let

$$\Theta(t) = \begin{cases} \Lambda \mathrm{e}^{-(\mathrm{t}-\mathrm{t_0})^2/\mathrm{T}^2}, & 0 \leq t \\ 0, & \text{otherwise} \end{cases}, \tag{S6}$$

with $\Lambda$ being the pumping rate. The length of the pulse is $T$ and the peak of the pulse is at time $t_0$.

Using the boundary condition $n_\mathrm{p,R}(\infty) = 0$ and $n_\mathrm{p,R}(0) = 0$, we find the solution for the first order linear differential equation of $n_\mathrm{p}$ as

$$n_\mathrm{p}(t) = \mathrm{e}^{-(\gamma_\mathrm{p}+\mathrm{r})\mathrm{t}} \int_0^\mathrm{t} \mathrm{e}^{(\gamma_\mathrm{p}+\mathrm{r})\mathrm{t}'} \Theta(t') dt' \tag{S7}$$

Therefore, for the time evolution of the exciton population in the reservoir, we have

$$n_\mathrm{R}(t) = r\mathrm{e}^{-\gamma_\mathrm{R}\mathrm{t}} \int_0^\mathrm{t} \mathrm{e}^{\gamma_\mathrm{R}\mathrm{t}'} n_\mathrm{p}(t') dt' \tag{S8}$$

These give the total excitons population as

$$n_\mathrm{X}(t) = n_\mathrm{p}(t) + n_\mathrm{R}(t) \tag{S9}$$

where $n_\mathrm{p}(t)$ and $n_\mathrm{R}(t)$ can be easily numerically evaluated using Eqs. (S7) and (S8).

## Comparison of the $\mathbf{X}_{\mathrm{A-BL}}$ and hIX cavity pumping

In this section, we use Eqs.(S3), (S7), and (S8) to simulate the time-resolve spectrum in Figs. S6a - S6c for $\mathrm{X}_{\mathrm{A-BL}}$ pumping and Fig.S6d for hIX pumping. In the $\mathrm{X}_{\mathrm{A-BL}}$ pumping, we find

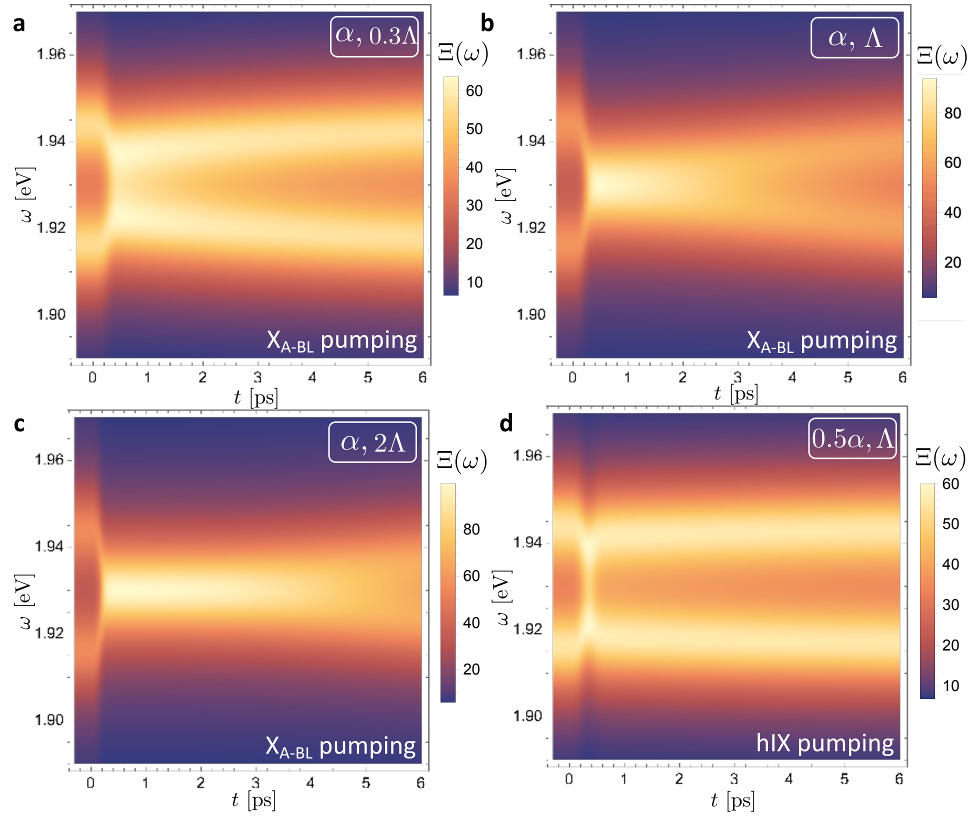


Supplementary Figure S6. a-c) Simulated pump fluence dependence of intralayer pumping. In this plot, we set $\gamma_{\rm p} = \gamma = 10$meV, $r = \gamma_{\rm p}$, and $\gamma_{\rm R} = 0.01\gamma_{\rm p}$. The insets of the upper right corner show the relative strength of the saturation effects $\alpha$ and the pumping rate $\Lambda$. The nominal value of these quantities is set to $\alpha = 0.05L^2$ and $\Lambda = 0.1L^{-2}$ps$^{-1}$ where $L^2$ being the size of the sample. The plots of $\Xi(\omega) = {\rm Im}[G_{\rm c}(\omega)]$ with pumping rate $0.3\Lambda$ in (a), $\Lambda$ in (b), and $2\Lambda$ in (c) demonstrate the excitation fluence dependence of the time-resolved spectrum. d) hIX pumping. Most of the parameters are the same as in (**a**) - (**c**) except we use a slightly longer lifetime for hIX with $\gamma_{\rm p} = 8$meV, smaller transferring rate $r = 0.1\gamma_{\rm p}$ to reservoir, and smaller saturation factor $0.5\alpha$.

a large portion of the pumped exciton transfer to the reservoir on the picosecond timescale [14]. This process is relevant only if the exciton lifetime is comparable to the transfer rate $r \approx \gamma_{\rm p}$. After all exciton transferring to the reservoir, the later nonlinear response is mostly determined by the long-lived state in the reservoir. This may explain the slower timescale in the SC recovery phase. In Fig. S6, we also simulate the excitation fluence dependence of the recovery time. The higher pump fluence leads to a longer recovery time since more long-lived excitons in the reservoir are created. Thus, the system requires a longer time to relax back to a lower exciton population to establish the SC phase. This trend is consistent with the experimental observation.

In contrast to the $X_{\rm A-BL}$ pumping case, by pumping the hIX the transfer rate to the reservoir is

slower ($r \approx 0.1\gamma_{\mathrm{p}}$). In such a case, a significant portion of the pumped hIX exciton recombines into photons before transferring into the reservoir. In the SC recovery phase, a much smaller long-lived exciton density remains in the reservoir. Additionally, the nonlinear saturation factor $\alpha$ is smaller due to the mitigation of blockade effects (see main text Fig.4a) leading to a faster recovery time of SC, see Fig. S6d.

As we discussed in the main text, transferring a momentum-bright into momentum-dark states can be achieved by scattering with the impurities and phonon. These scattering may gives a smaller $r$ in hIX. Particularly, hIX has weaker scattering with impurities due to the wavefunction spreading in the out-of-plane direction. Also, interacting with phonon, this can also lead to thermal relaxation that transfers the (high-energy) bright state and dark (low-energy) states. However, in a thermal process the rate $r$ depends on the relative energies separation ($\Delta$) between the high-energy state and low-energy states. The smaller of the energy separation results in smaller $r$, since thermal fluctuations allow the opposite transition from low-energy to high-energy states. The transition amplitude of this adverse effects is roughly given by the Boltzmann factor $\mathrm{e}^{-\Delta/(\mathrm{k_B T})}$. In small $\Delta$ case, the low-to-high energy transition may not be strongly suppressed and reverse the relaxation process in converting the bright states to the reservoir leading to a smaller $r$. As suggested in Ref. [15], there exist many low energy momentum-dark states for hIX which are potentially close to the bright hIX. The transition between these states may has a smaller $r$. However, to be more conclusive, we note that the transition between these states in Ref. [15] due to the scattering with impurities and phonon required further detailed investigations.

## SUPPLEMENTARY NOTE S7: DOUBLE BILAYER MICROCAVITY

To form a double BL cavity two bilayers were overlapped on the bottom DBR to make a double bilayer structure with a separation of 40 nm of hBN between them. The cavity was again completed by a PMMA spacer and silver mirror with the same thicknesses used for the single BL cavity. We measure the cavity reflectivity spectra as a function of the angle and for each angle we fit the spectrum with Lorentzians. The extracted peak energies are then fitted with a three-level coupled oscillators model, such that

$$H_{\mathrm{DBL}} = \begin{pmatrix} E_{\mathrm{c}} & \Omega_{\mathrm{A_{DBL}}} & \Omega_{\mathrm{hIX_{DBL}}} \\ \Omega_{\mathrm{A_{DBL}}} & E_{\mathrm{A_{DBL}}} & 0 \\ \Omega_{\mathrm{hIX_{DBL}}} & 0 & E_{\mathrm{hIX_{DBL}}} \end{pmatrix}$$

As can be seen in Fig S7, two anticrossings can be observed at the energies of $\mathrm{X_A}$ and hIX. The

latter are at 1.932 and 1.992 eV for $A_{DBL}$ and $hIX_{DBL}$, respectively, with a slight redshift of both excitons by 8 meV, with the intra to interlayer exciton energy separation being consistent with the single bilayer case. The cavity has a negative detuning of 11 meV from $A_{DBL}$. The corresponding Rabi splittings are extracted as $\Omega_{A_{DBL}} = 55.0 \pm 0.5$ meV and $\Omega_{hIX_{DBL}} = 31.8 \pm 0.9$ meV.

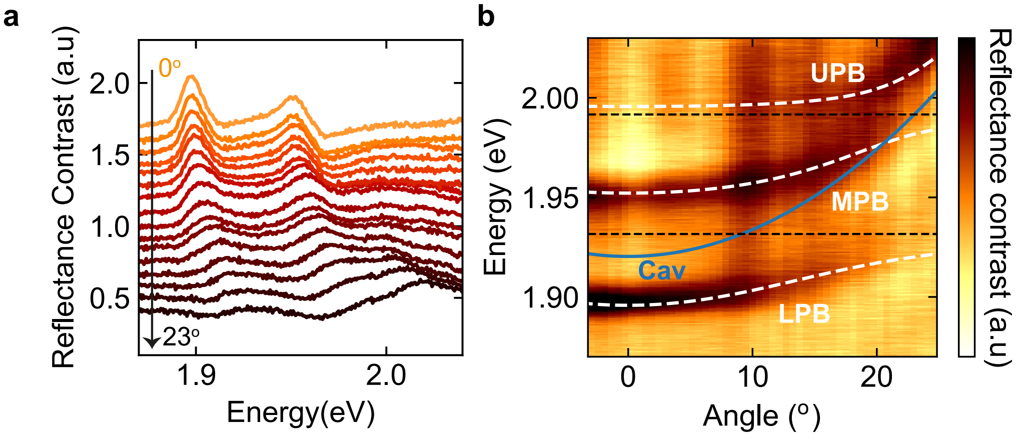


Supplementary Figure S7. a) Waterfall plot of the RC spectra as a function of angle for a double bilayer $MoS_2$ embedded in a microcavity. Two anticrossings are observed at the $X_A$ and hIX energies, respectively. b) Energy-angle map of the cavity reflectivity spectra. The fitted Upper, Middle and Lower polariton branches (UPB, MPB, LPB) are shown as white dashed curves. The cavity mode (Cav) is shown as a blue solid curve, whereas the exciton energies are shown as black dashed lines.

---

* Contributed equally

† a.tartakovskii@sheffield.ac.uk

‡ giulio.cerullo@polimi.it

[1] Z. Nie, R. Long, L. Sun, C.-C. Huang, J. Zhang, Q. Xiong, D. W. Hewak, Z. Shen, O. V. Prezhdo, and Z.-H. Loh, Ultrafast carrier thermalization and cooling dynamics in few-layer mos2, ACS nano **8**, 10931 (2014).

[2] N. U. Din, V. Turkowski, and T. S. Rahman, Ultrafast charge dynamics and photoluminescence in bilayer mos2, 2D Materials **8**, 025018 (2021).

[3] F. Katsch, M. Selig, and A. Knorr, Exciton-scattering-induced dephasing in two-dimensional semiconductors, Physical Review Letters **124**, 257402 (2020).

[4] Y. Tang, Y. Zhang, Q. Liu, K. Wei, X. Cheng, L. Shi, and T. Jiang, Interacting plexcitons for designed ultrafast optical nonlinearity in a monolayer semiconductor, Light: Science & Applications **11**, 94 (2022).

[5] S. J. Byrnes, Multilayer optical calculations, arXiv preprint arXiv:1603.02720 (2016).

[6] S. Calati, Q. Li, X. Zhu, and J. Stähler, Ultrafast evolution of the complex dielectric function of monolayer ws 2 after photoexcitation, Physical Chemistry Chemical Physics **23**, 22640 (2021).

[7] D. J. Gillard, A. Genco, S. Ahn, T. P. Lyons, K. Yeol Ma, A. R. Jang, T. Severs Millard, A. A. Trichet, R. Jayaprakash, K. Georgiou, D. G. Lidzey, J. M. Smith, H. Suk Shin, and A. I. Tartakovskii, Strong exciton-photon coupling in large area $MoSe_2$ and $WSe_2$ heterostructures fabricated from two-dimensional materials grown by chemical vapor deposition, 2D Materials **8** (2021).

[8] D. Golla, K. Chattrakun, K. Watanabe, T. Taniguchi, B. J. LeRoy, and A. Sandhu, Optical thickness determination of hexagonal boron nitride flakes, Applied Physics Letters **102** (2013).

[9] A. Kuzmenko, Kramers–kronig constrained variational analysis of optical spectra, Review of scientific instruments **76** (2005).

[10] Y. Li, A. Chernikov, X. Zhang, A. Rigosi, H. M. Hill, A. M. Van Der Zande, D. A. Chenet, E.-M. Shih, J. Hone, and T. F. Heinz, Measurement of the optical dielectric function of monolayer transition-metal dichalcogenides: Mos 2, mo s e 2, ws 2, and ws e 2, Physical Review B **90**, 205422 (2014).

[11] F. Huang, Optical contrast of atomically thin films, The Journal of Physical Chemistry C **123**, 7440 (2019).

[12] C. Louca, A. Genco, S. Chiavazzo, T. P. Lyons, S. Randerson, C. Trovatello, P. Claronino, R. Jayaprakash, X. Hu, J. Howarth, et al., Interspecies exciton interactions lead to enhanced non-linearity of dipolar excitons and polaritons in mos2 homobilayers, Nature Communications **14**, 3818 (2023).

[13] K. W. Song, S. Chiavazzo, and O. Kyriienko, Microscopic theory of nonlinear phase space filling in polaritonic lattices, Physical Review Research **6**, 023033 (2024).

[14] M. Selig, G. Berghäuser, A. Raja, P. Nagler, C. Schüller, T. F. Heinz, T. Korn, A. Chernikov, E. Malic, and A. Knorr, Excitonic linewidth and coherence lifetime in monolayer transition metal dichalcogenides, Nature Communications **7**, 13279 (2016).

[15] T. Deilmann and K. S. Thygesen, Finite-momentum exciton landscape in mono- and bilayer transition metal dichalcogenides, 2D Materials **6**, 035003 (2019).
